# Supplementary material for: Decontextualization: Making Sentences Stand-Alone
Source: arXiv:2102.05169 source file (2021-02-09)
Supplement: Supplementary file 1 [file appendix.tex]

\section{Appendices}

\begin{figure*}

\caption{Instruction shown to the annotators of the task.}\label{fig:annotation}
\end{figure*}
\label{sec:appendix}
